# Supplementary material for: Dynamic Power Splitting for SWIPT with Nonlinear Energy Harvesting in Ergodic Fading Channel
Source: arXiv:1804.07398 source file (2018-08-27)
Supplement: Supplementary file 1 [file appendix_proof_thm_2.tex]

\section{Proof of Theorem \ref{thm_2}}
\label{proof_thm_2}

The Lagrange dual function for (P1') is given by 
\begin{align}
\label{C1}
\mathcal{D}' ( \lambda )  =  \underset{  0 \leq \rho_{\nu} \leq 1 , \forall \nu  }{\texttt{max}} & ~ \mathbb{E} \left[ (1 - \rho_{\nu}) R_{\nu} (  P_{\rm avg} , 0  )  \right] \nonumber\\
& ~ + \lambda  \left( \mathbb{E} \left[  Q_{\nu}^{\texttt{NL}} (  P_{\rm avg} , \rho_{\nu}  )  \right] - Q \right)
\end{align}
where $\lambda$ is the dual variable associated with the average harvested energy constraint of (\ref{P1_const_1_}).
Similarly as in Appendix \ref{proof_thm_1}, 
it can be shown that the optimal dual variable $\lambda^{\texttt{NL}}$ is determined to satisfy the average harvested energy constraint with equality, i.e., $ \mathbb{E} \left[  Q_{\nu}^{\texttt{NL}} (  P_{\rm avg} , \rho_{\nu}^{*}  )  \right] = Q$, where $ \rho_{\nu}^{*} $ denotes the solution to (\ref{C1}).
Thus, in the following, we focus on the proof of the solution $ \rho_{\nu}^{*} $ to (\ref{C1}) given the dual variable $\lambda$.

Given $\lambda$, the problem of (\ref{C1}) can be decoupled into parallel subproblems, each for one particular fading state $\nu$, as follows:
\begin{align}
\label{C2}
\underset{ 0 \leq \rho_{\nu}  \leq 1 }{\max}  \quad  \mathcal{L}_{\nu}' ( \rho_{\nu} )
\end{align}
where
\begin{align}
\label{C3}
\mathcal{L}_{\nu}' ( \rho_{\nu} )  =  (1 - \rho_{\nu}) R_{\nu} ( P_{\rm avg}, 0 ) + \lambda  Q_{\nu}^{\texttt{NL}} ( P_{\rm avg}, \rho_{\nu} ) .
\end{align}
The KKT conditions are given by 
\begin{align}
\label{C4}
\frac{\partial \mathcal{L}_{\nu}'}{\partial \rho_{\nu}} & =  \begin{cases}  \leq 0,  &  {\rm if} ~ \rho_{\nu}^{*} = 0 \\ \geq 0,  &  {\rm if} ~ \rho_{\nu}^{*} = 1 \\   = 0,  &  {\rm if} ~ 0 < \rho_{\nu}^{*} < 1  \end{cases}
\end{align}
where 
\begin{align}
\label{C5}
\frac{\partial \mathcal{L}_{\nu}'}{\partial \rho_{\nu}} & = \lambda \frac{ P_{s} T a h_{\nu} P_{\rm avg}  \Psi_{\nu} ( P_{\rm avg}, \rho_{\nu}  ) \left(  1 - \Psi_{\nu} ( P_{\rm avg}, \rho_{\nu}  ) \right) }{ 1 - \Omega }
\nonumber\\
& \quad - R_{\nu} ( P_{\rm avg}, 0 ).
\end{align}

First, we derive the solution for the Case 1'. Since $\Psi_{\nu} ( P_{\rm avg}, \rho_{\nu}  ) \left(  1 - \Psi_{\nu} ( P_{\rm avg}, \rho_{\nu}  ) \right) \leq\frac{1}{4}$ for $\forall 0 \leq \rho_{\nu} \leq 1$,
it follows from (\ref{C5}) that if $\lambda \frac{ P_{s} T a h_{\nu} P_{\rm avg}   }{ 4 ( 1 - \Omega ) } \leq R_{\nu} ( P_{\rm avg}, 0 )$, or equivalently, $z ( h_{\nu} ) \geq  \frac{\lambda^{\texttt{NL}}}{4} $,
then $ \frac{\partial \mathcal{L}_{\nu}'}{\partial \rho_{\nu}} \leq 0 $.
Thus, from (\ref{C4}), we have $\rho_{\nu}^{*} = 0$ for the Case 1' when $z ( h_{\nu} ) \geq  \frac{\lambda^{\texttt{NL}}}{4} $.

Next, we consider the case when $z ( h_{\nu} ) <  \frac{\lambda^{\texttt{NL}}}{4} $.
From (\ref{C4}) and (\ref{C5}), we have
\begin{align}
\label{C6}
\lambda f ( 0 ) \leq z ( h_{\nu} ),  & \quad   {\rm if} ~ \rho_{\nu}^{*} = 0  \\
\label{C7}
\lambda f ( h_{\nu} ) \geq  z ( h_{\nu} ),  & \quad   {\rm if} ~ \rho_{\nu}^{*} = 1 .
\end{align}
Also, solving the equation $ \frac{\partial \mathcal{L}_{\nu}'}{\partial \rho_{\nu}} = 0 $, we can obtain the value of $0 < \rho_{\nu}^{*} < 1$.
Since the equation $ \frac{\partial \mathcal{L}_{\nu}'}{\partial \rho_{\nu}} = 0 $ is quadratic in $\Psi_{\nu} (\cdot)$,
it has two roots. One is the local minimum, given by $ \Psi_{\nu}^{\rm } ( P_{\rm avg}, \rho_{\nu}  ) =  \frac{1}{2} - \sqrt{ \frac{1}{4} - \frac{z(h_{\nu})}{\lambda} } $.
The other is the local maximum, given by $ \Psi_{\nu}^{\rm } ( P_{\rm avg}, \rho_{\nu}  ) =  \frac{1}{2} + \sqrt{ \frac{1}{4} - \frac{z(h_{\nu})}{\lambda} } $.
Solving this equation with respect to $\rho_{\nu}$, the local maximum can be obtained as $ \rho_{{\rm so}, \nu}  =  \frac{1}{h_{\nu} P_{\rm avg}} \left( - \frac{1}{a}  \ln \left(  \frac{ 2 }{  1 + \sqrt{ 1 - \frac{ 4 z ( h_{\nu} ) }{ \lambda } }  } - 1 \right) + b \right) $, which is the solution of the equation $ \frac{\partial \mathcal{L}_{\nu}'}{\partial \rho_{\nu}} = 0 $, i.e., $ \rho_{\nu}^{*} = \rho_{{\rm so}, \nu}$.
It follows from (\ref{C4}) and (\ref{C5}) that if $ \left. \frac{\partial \mathcal{L}_{\nu}'}{\partial \rho_{\nu}} \right|_{\rho_{\nu} = 1} $, or equivalently, $\lambda f ( h_{\nu} ) <  z ( h_{\nu} )$, then $0 < \rho_{\nu}^{*} < 1$. From this, we have 
\begin{align}
\label{C8}
\lambda f ( h_{\nu} ) <  z ( h_{\nu} ),  & \quad   {\rm if} ~ 0 < \rho_{\nu}^{*} < 1 .
\end{align}
In the following, when we derive the solution to (\ref{C2}) for the four possible cases of the functions $f(\cdot)$ and $z(\cdot)$.
\begin{enumerate} [label=\textit{\roman*}')]
\item $ \lambda f ( 0 ) \leq z ( h_{\nu} ) $ and $\lambda f ( h_{\nu} )  <  z ( h_{\nu} )$: In this case, both the conditions (\ref{C6}) and (\ref{C8}) are satisfied. Thus, the solution can be either $\rho_{\nu}^{*} = 0$ or $\rho_{\nu}^{*} = \rho_{{\rm so}, \nu}$. To obtain the solution, we need to compare the two objective values: $\mathcal{L}_{\nu} ( 0 )$ and $\mathcal{L}_{\nu} ( \rho_{{\rm so}, \nu} )$. If $\mathcal{L}_{\nu} (  \rho_{{\rm so}, \nu} ) > \mathcal{L}_{\nu} ( 0 )$, or equivalently, $R_{\nu} ( P_{\rm avg}, \rho_{{\rm so}, \nu} )  + \lambda Q_{\nu}^{\texttt{NL}} ( P_{\rm avg}, \rho_{{\rm so}, \nu} ) >  R_{\nu} ( P_{\rm avg} , 0 ) $, the solution is given by $\rho_{\nu}^{*} =  \rho_{{\rm so}, \nu}$. Otherwise, the solution is given by $\rho_{\nu}^{*} = 0$.

\item $ \lambda f ( 0 ) \leq z ( h_{\nu} ) $ and $\lambda f ( h_{\nu} )  \geq  z ( h_{\nu} )$: In this case, both the conditions (\ref{C6}) and (\ref{C7}) are satisfied. Thus, the solution can be either $\rho_{\nu}^{*} = 0$ or $\rho_{\nu}^{*} = 1$. To obtain the solution, we need to compare the two objective values: $\mathcal{L}_{\nu} (  0 )$ and $\mathcal{L}_{\nu} (  1 )$. If $\mathcal{L}_{\nu} (  1 ) > \mathcal{L}_{\nu} (  0 ) $, or equivalently, $\lambda Q_{\nu}^{\texttt{NL}} ( P_{\rm avg} , 1 ) >  R_{\nu} ( P_{\rm avg} , 0 )$, the solution is given by $\rho_{\nu}^{*} = 1$. Otherwise, the solution is given by $\rho_{\nu}^{*} = 0$.

\item $ \lambda f ( 0 ) > z ( h_{\nu} ) $ and $\lambda f ( h_{\nu} )  <  z ( h_{\nu} )$: In this case, only the condition (\ref{C8}) is satisfied. Thus, the solution is given by $\rho_{\nu}^{*} =  \rho_{{\rm so}, \nu}$.

\item $ \lambda f ( 0 ) > z ( h_{\nu} ) $ and $\lambda f ( h_{\nu} )  \geq  z ( h_{\nu} )$: In this case, only the condition (\ref{C7}) is satisfied. Thus, the solution is given by $\rho_{\nu}^{*} = 1$.
\end{enumerate}

The above cases \textit{i')}--\textit{iv')} can be equivalently written as the Cases 2'--5' as in (\ref{rho_NL_so_cases}).
Thus, the solutions obtained for the above cases \textit{i')}--\textit{iv')} correspond to those for the Cases 2'--5', respectively.
